# Supplementary material for: An Empirical Analysis of Range for 3D Object Detection
Source: arXiv:2308.04054 source file (2023-08-08)
Supplement: Supplementary file 1 [file suppl.tex]

%%%%%%%%% ABSTRACT
\begin{center}
    \Large
    \textbf{Outline} 
\end{center}
In this supplementary document, we present results on the nuScenes dataset, further analyze model run time, and provide additional analysis on Argoverse 2.0 results presented in the main paper. Importantly, we find that building range experts is not effective at close range (particularly for nuScenes). Further, we find that the point-processing is a significant bottleneck across all models, suggesting that a shared encoder across range experts can provide considerable efficiency gains. Lastly, we show that our analysis on the impact of network architecture and training losses for across-range generalization holds for a new detector. 

\appendix
\section{Evaluating on nuScenes}

%\begin{figure}
%    \centering
%    \includegraphics[width=\linewidth]{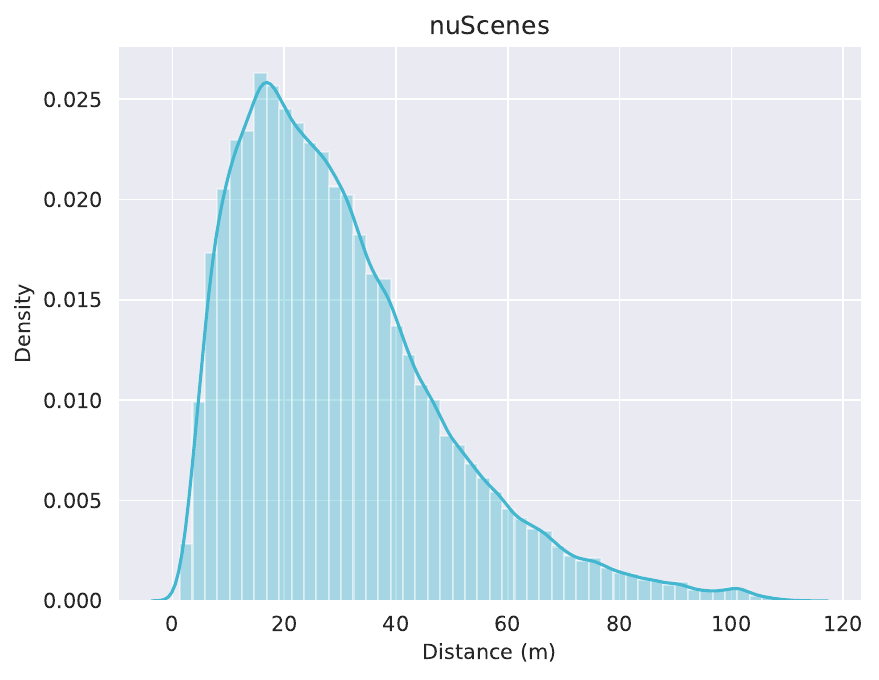}
%    \caption{Data augmentation due to data between 25-50m. }
%    \label{fig:my_label}
%\end{figure}
We evaluate the performance of PointPillars \cite{lang2019pointpillars}, CBGS \cite{zhu2019class}, and CenterPoint \cite{yin2021center} on the nuScenes dataset. Although our primary focus is long-range detection, we evaluate short-range detection for completeness. 

\textbf{Dataset and Metrics}. 
Although nuScenes annotates 23 classes, it only evaluates on 10 common classes like {\tt car} and {\tt pedestrian}. To more closely resemble the long-tailed ontology of Argoverse 2.0, we follow the protocol used by \cite{peri2022lt3d} to evaluate on 18 classes, which includes more diverse classes like {\tt stroller} and {\tt debris}.  We evaluate the performance of our detector on all classes at both 0-25m and 0-50m. We adopt 10-frame aggregation for LiDAR densification. We assume that we are provided with ego-vehicle pose for prior frames to align all LiDAR sweeps to the current ego-vehicle pose. Since LiDAR returns are sparse, this densification step is commonly used.

We evaluate all methods using the nuScenes Detection Score (NDS), which is comprised of mAP and five true-positive metrics, including average translation error, average orientation error, average scale error, average velocity error, and average attribute error. For 3D detection on LiDAR sweeps, a true positiveis defined as a detection that has a center distance within a distance threshold on the ground-plane to a ground-truth annotation. mAP computes the mean of AP over classes, where per-class AP is the area under the precision-recall curve, and distance thresholds of $[0.5, 1, 2, 4]$ meters.  NDS is defined as the weighted sum of mAP and the true-positive metrics. We refer readers to \cite{caesar2020nuscenes} for further details about the metrics. 
\begin{table}[b]
\small
\centering
\caption{{\bf nuScenes Evaluation Results}. We evaluate three popular LiDAR-based 3D detectors on the nuScenes dataset. Similar to Argoverse 2.0, we breakdown evaluation into two cohorts: 0-25m and 0-50m. We find that there is no benefit in training range experts for short-range detection. Specifically, training models for 50m yields the best performance when evaluating at both 25m or 50m. We posit that the 25m range expert performs worse than the 50m range expert simply because it sees half as many examples. 
}
\label{tab:nus}
\adjustbox{width=\linewidth}{
\begin{tabular}{@{}cclcccccccc@{}}
\toprule
ID & \multicolumn{1}{c}{Model} & \multicolumn{1}{c}{Method}   & 0-25m         & 0-50m      \\ \midrule
1 & PointPillars & 25/16 → 25   &  47.8           &   40.3   \\
2 &  & 25/16 → 50   &    47.9         &    41.9              \\
3 &  & 50/8 → 25 &       50.3    &     41.8                  \\
4 &  & 50/8 → 50 &    {\bf 50.6}       &    {\bf 46.0}       \\ \midrule
1 & CBGS & 25/25 → 25   &   50.6          &   42.9           \\
2 &  & 25/25 → 50   &    50.0         &    43.2              \\
3 &  & 50/12.5 → 25 &   48.8       &    41.4                 \\
4 &  & 50/12.5 → 50 &   {\bf 51.0}        &    {\bf 45.2}     \\ \midrule
1 & CenterPoint & 25/25 → 25   &   56.3          &   46.9     \\
2 &  & 25/25 → 50   &   55.9          &    48.0        \\
3 &  & 50/12.5 → 25 &   55.4        &   46.0         \\
4 &  & 50/12.5 → 50 &   {\bf 56.5}        &    {\bf 48.9}        \\ \bottomrule
%1 & TransFusion & 25/25 → 25   &             &           \\
%2 &  & 25/25 → 50   &             &            &             \\
%3 &  & 50/12.5 → 25 &           &            &              \\
%4 &  & 50/12.5 → 50 &           &            &              \\ \bottomrule
\end{tabular}
} % adjustbox
\end{table}

{\bf Short Range Evaluation}. We train on data between 0-25m and 0-50m, and evaluate models on LiDAR-sweeps between 0-25m and 0-50m using fully convolutional processing in Table \ref{tab:nus}. Unlike Argoverse 2.0, where different range / voxel size combinations allowed for range experts and ensembles, we find that the best performing models were trained and evaluated on 50m. Surprisingly, using a finer-grained voxel size when training the 25m models does not lead to better performance in the 0-25m range for any of the models, suggesting that fine-grained voxel processing may not always result in the best performance. 
%%%%%%%%%
% METRICS
%%%%%%%%%

\begin{table*}[t]
\small
\centering
\adjustbox{width=\linewidth}{
\setlength{\tabcolsep}{5pt}
\begin{tabular}{@{}cllccccccc@{}}
\toprule
ID & Model & \multicolumn{1}{c}{Method} & Point Proc.      & Backbone  & Neck & Head & Post Proc. \\ \midrule
1  & PointPillars & 50/4 → 50    &   10.5 $\pm$ 3.0         &   3.5 $\pm$ 0.2         &   1.9 $\pm$ 0.1       &   1.2 $\pm$ 0.1        &  58.2 $\pm$ 1.6             \\ 
2  & CBGS &  50/12.5 → 50            &    43.6 $\pm$ 4.0       &   4.7 $\pm$ 0.3         &   2.5 $\pm$ 0.1       &   1.2  $\pm$ 0.2        &   55.9 $\pm$ 3.5             \\
3  & CenterPoint & 50/12.5 → 50     &    45.8 $\pm$  5.5      &   2.7 $\pm$ 0.3       &   0.8 $\pm$ 0.03       &  42.8 $\pm$ 0.6         &   440.9 $\pm$ 48.1           \\
4  & TransFusion-L & 50/12.5 → 50     &   264.9 $\pm$ 45.8         &     4.5 $\pm$ 0.2       &    1.3 $\pm$ 0.3      &   9.8 $\pm$ 3.4        &    1.5 $\pm$ 0.5             \\ \midrule
1  & PointPillars & 100/4 → 100    &   25.6 $\pm$ 7.3         &   10.6 $\pm$ 0.1         &   13.1 $\pm$ 0.1       &   4.1 $\pm$ 0.1        &  62.0 $\pm$ 1.3             \\ 
2  & CBGS &  100/6.25 → 100            &    40.0 $\pm$ 3.2       &   4.7 $\pm$ 0.1         &   2.5 $\pm$ 0.1       &   1.2  $\pm$ 0.1        &   58.6 $\pm$ 1.9             \\
3  & CenterPoint & 100/6.25 → 100     &    42.3 $\pm$  6.1      &   4.8 $\pm$ 0.2       &   0.8 $\pm$ 0.1       &  42.7 $\pm$ 0.6         &   448.1 $\pm$ 54.8           \\
4  & TransFusion-L & 100/6.25 → 100     &    257.7 $\pm$ 34.9                   &      4.5 $\pm$ 0.4                 &    1.3 $\pm$  0.1          &    9.3 $\pm$  2.6       &     1.5 $\pm$  0.2         \\ \midrule
1  & PointPillars & 150/2 → 150    &       4.0  $\pm$ 1.2             &    6.6 $\pm$ 0.3                   &   8.1 $\pm$ 0.2           &   2.7 $\pm$ 0.3        &    60.0 $\pm$ 9.1          \\
2  & CBGS &  150/3.125 → 150           &  35.5 $\pm$ 1.9                    &     3.0 $\pm$ 0.1                  &    1.7 $\pm$ 0.1          &   1.1 $\pm$ 0.1        &   58.8 $\pm$ 1.5           \\
3  & CenterPoint & 150/3.125 → 150     &     33.5 $\pm$ 4.4                 &     3.3 $\pm$ 0.2                  &    0.6 $\pm$ 0.1          &    26.1 $\pm$ 1.0       &   291.1 $\pm$ 66.9           \\    
4  & TransFusion-L & 150/3.125 → 150     &   240.9  $\pm$ 31.6                   &     3.3 $\pm$  0.7                  &     0.8 $\pm$  0.1         &    9.0 $\pm$ 2.1       &      1.5 $\pm$  0.5        \\ \bottomrule

\end{tabular}
} % \adjustbox
\caption{\textbf{Impact of Range on Timing}. We find that increasing range and proportionally decreasing voxel resolution keeps run time approximately constant. Within a fixed compute budget, tuning range and voxel resolution are the two key ``knobs'' to trade off latency and accuracy. Further, we find that the point-processing takes a majority of the run time (excluding post-processing). Lastly, we note that CenterPoint's head is more than four times slower than the transformer head in TransFusion and ten times slower than the anchor head in PointPillars. Empirically, we find that this slowdown is due to inefficient bounding box decoding from the CenterPoint regression heads (which can be significanlty optimized). 
}
\label{tab:runtime-long-range}
\end{table*}

\begin{table*}[t]
\small
\centering
\adjustbox{width=\linewidth}{
\setlength{\tabcolsep}{5pt}
\begin{tabular}{@{}cllccccccc@{}}
\toprule
ID & Model & \multicolumn{1}{c}{Method} & {\bf Point Proc.}      & Backbone  & Neck & Head & Post Proc. \\ \midrule
1  & PointPillars (spconv1.0) & 50/4 → 50    &     {\bf 33.1  $\pm$ 4.4}       &    10.6 $\pm$ 0.1         &    13.1 $\pm$ 0.1       &   4.1 $\pm$ 0.1         &    60.5 $\pm$ 5.5            \\ 
2  & CBGS (spconv1.0) &  50/12.5 → 50            &     {\bf 64.4 $\pm$ 7.2}       &    4.7 $\pm$ 0.1         &    2.5 $\pm$ 0.1       &   1.2 $\pm$ 0.1         &    45.4 $\pm$ 5.9            \\ 
3  & CenterPoint (spconv1.0) & 50/12.5 → 50     &   {\bf 66.8 $\pm$ 9.3}          &    2.7 $\pm$ 0.6         &    0.8 $\pm$ 0.1       &    42.6 $\pm$ 0.7        &     380.3 $\pm$ 45.9           \\  \midrule
1  & PointPillars (spconv2.0) & 50/4 → 50    &   {\bf 10.5 $\pm$ 3.0}         &   3.5 $\pm$ 0.2         &   1.9 $\pm$ 0.1       &   1.2 $\pm$ 0.1        &  58.2 $\pm$ 1.6             \\ 
2  & CBGS (spconv2.0)&  50/12.5 → 50            &    {\bf 43.6 $\pm$ 4.0}       &   4.7 $\pm$ 0.3         &   2.5 $\pm$ 0.1       &   1.2  $\pm$ 0.2        &   55.9 $\pm$ 3.5             \\
3  & CenterPoint (spconv2.0) & 50/12.5 → 50     &    {\bf 45.8 $\pm$  5.5}      &   2.7 $\pm$ 0.3       &   0.8 $\pm$ 0.03       &  42.8 $\pm$ 0.6         &   440.9 $\pm$ 48.1           \\ \bottomrule
\end{tabular}
} % \adjustbox
\caption{\textbf{Impact of Software Version on Timing}. Surprisingly, we find that the specific version of spconv used for sparse convolutions (in the point-processing and voxel encoding stage) can have a considerable impact on efficiency, accounting for nearly all of the difference in run time. Specifically, spconv 2.0 is 33\% faster than spconv1.0. 
}
\label{tab:runtime-spconv}
\end{table*}

\section{Run Time Analysis}
We identify the run time bottlenecks across models and show that point-processing accounts for a majority of the latency regardless of voxel size or detection range.

\textbf{Impact of Range on Timing}
We find two trends when analyzing the effect of range on latency, as shown in Table \ref{tab:runtime-long-range}. First, evaluating a model on longer-range inputs through fully-convolutional processing always increases latency. This is unsurprising, and analogous to increasing the image resolution in 2D detector architectures. Concretely, as feature maps increase in size when processing longer-range inputs, all sub-components in the model are slower. Next, we find that increasing range and proportionally decreasing voxel resolution keeps run time relatively constant. 

\textbf{Impact of Software Version on Timing}. We find that software versions within mmdetection3d (and its dependencies, mmdetection and mmcv) and spconv significantly influence latency. We evaluate PointPillars, CBGS, and CenterPoint in Table \ref{tab:runtime-spconv} and find that the voxel encoder for is up to 33\% slower with spconv 1.0. As the voxel encoder has a considerable impact on overall run time, these minor environment differences can result in significant differences in benchmarking. We use mmdetection3d 1.0.0rc4, mmdetection 2.28.0, mmcv 1.6.1, CUDA 11.3 and PyTorch 1.10.1. 

\section{Argoverse 2.0 Results}
We refer readers to the captions in Tables \ref{tab:av2-pointpillars-landscape}, \ref{tab:av2-cbgs-landscape}, \ref{tab:av2-centerpoint-landscape}, \ref{tab:av2-transfusion-landscape} for model-specific analysis.

\begin{figure*}[t]
    \centering
    \includegraphics[width=0.4 \linewidth, clip, trim={8cm 6cm 8cm 1.5cm}]{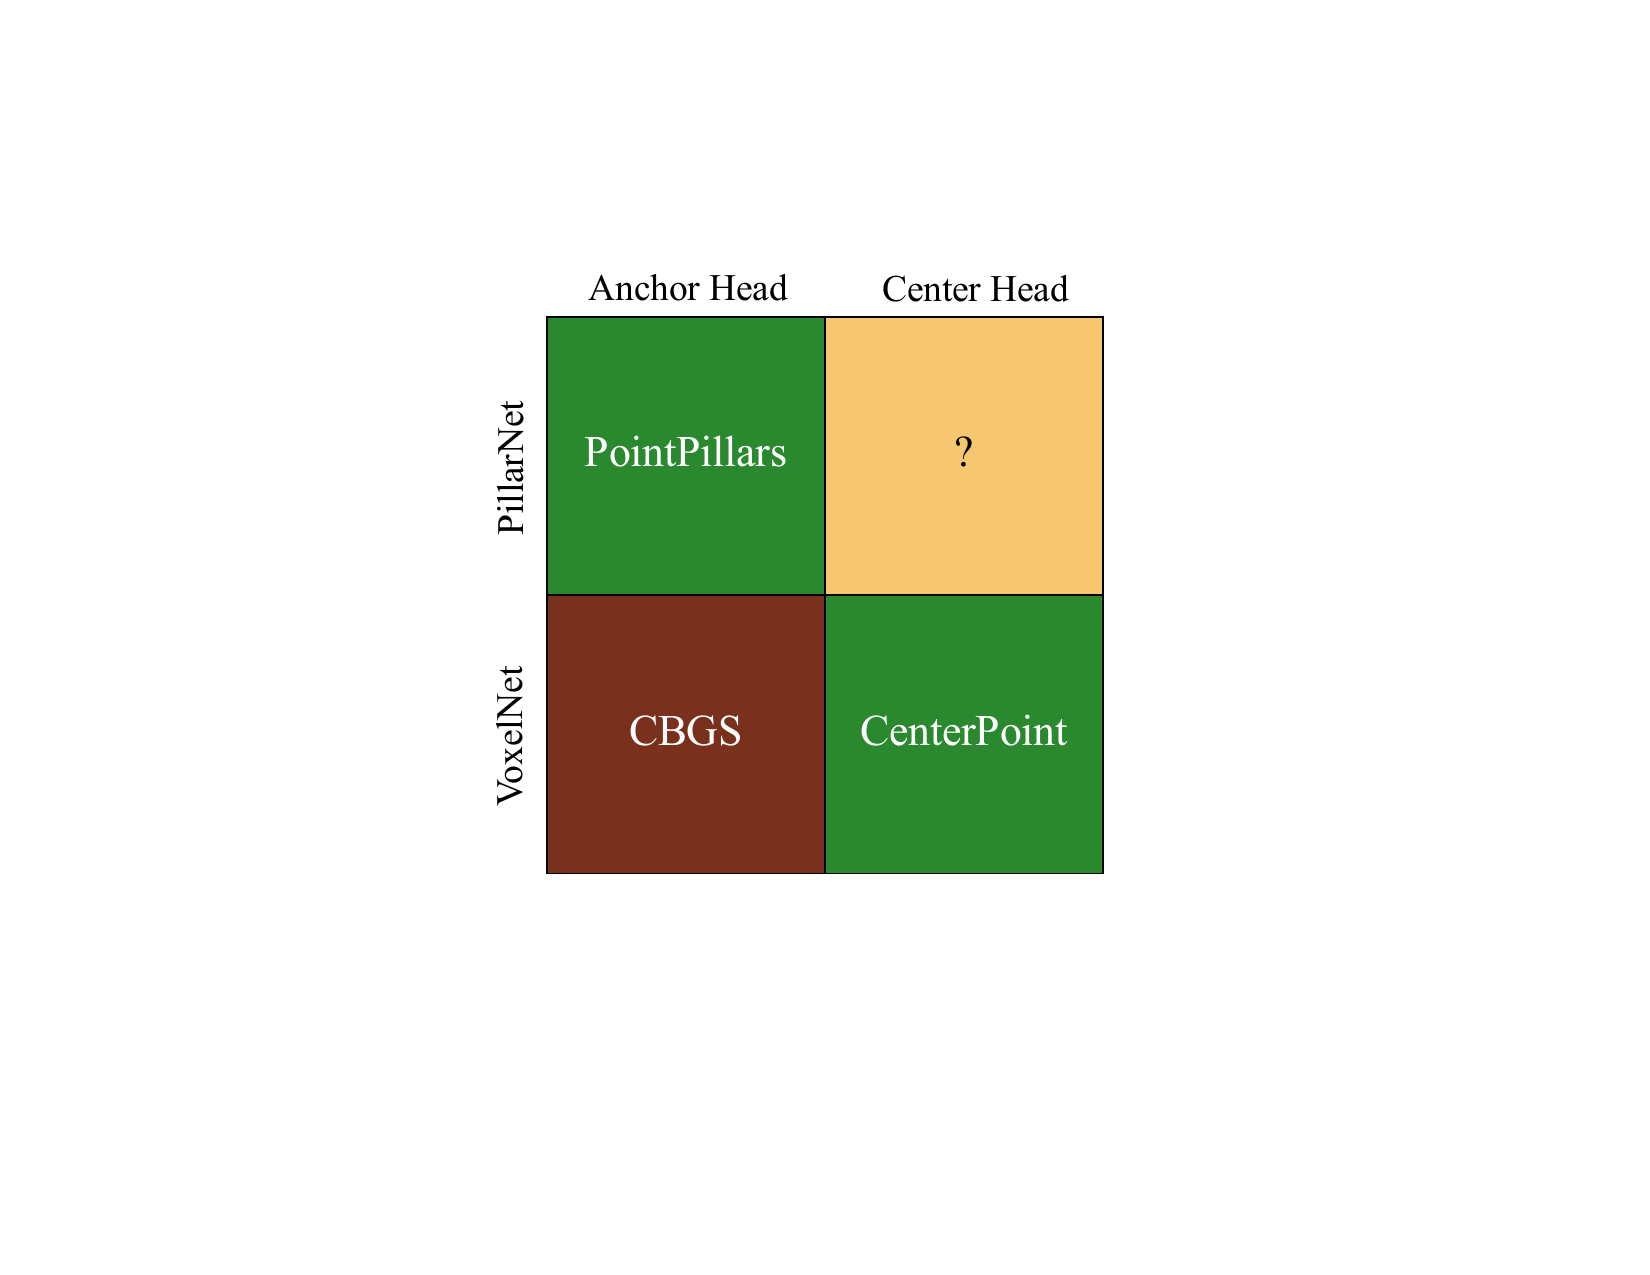}
    \includegraphics[width=0.4 \linewidth]{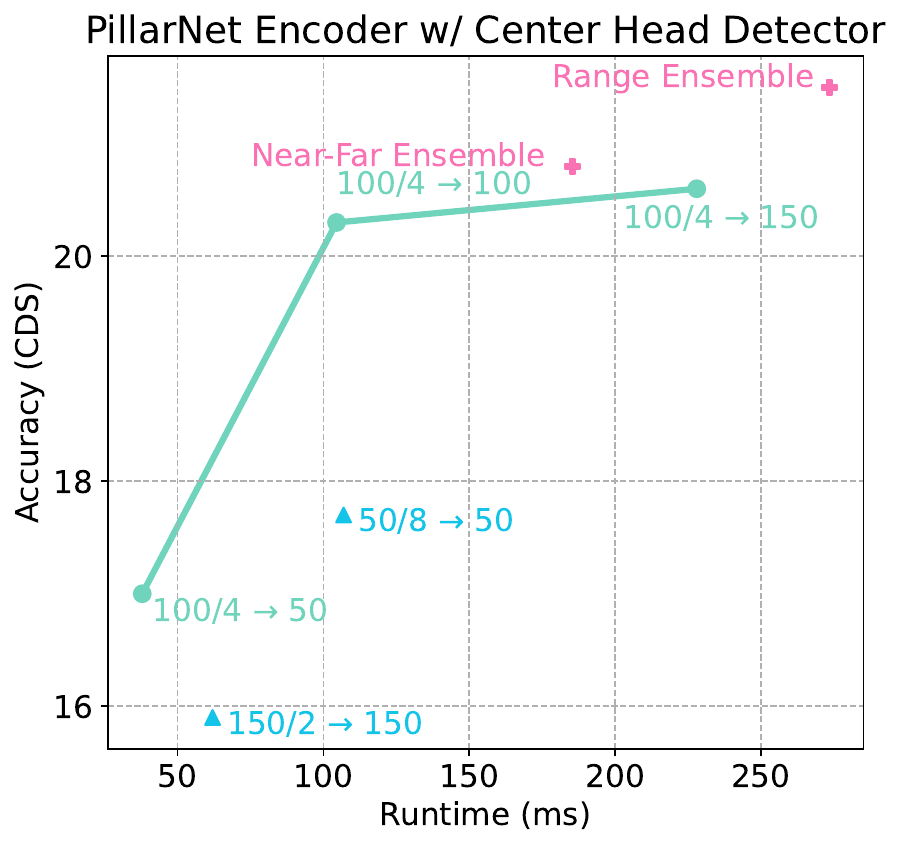}
    \caption{We evaluate the impact of model architecture and training loss on across-range generalization. We show that PointPillars (PillarNet + anchor head) and CenterPoint (VoxelNet + center head) generalize well beyond their training range. We evaluate a new model that uses a PillarNet encoder and a center head detector, and find that this model generalizes well across-range. We posit that the local features extracted from PillarNet and the soft-targets from the center head loss result in improved generalization across-range}
    \label{fig:novel}
\end{figure*}

\begin{table*}[t]
\small
\centering
\caption{{\bf PillarNet Encoder w/ Center Head Detector}. Based on prior trends with PointPillars and CenterPoint, we expect that a model trained with a PillarNet encoder and a center head detector to generalize well across range. Evaluating both the 100m (visualized in Fig. \ref{fig:novel}) and 150m range experts, we find that both models generalize across-range. Specifically, we see that for the 100m range expert, the performance of the 0-50m and 50-100m are consistent (rows 4 - 6). In contrast, we find that the  50m range expert does not generalize well, suggesting that across-range generalization is both a property of training range and voxel size. Concretely, training only with dense near-field LiDAR points or fine-grained voxels won't generalize well at long-range with sparse LiDAR-points. Finally, we note that the near-far ensemble (row 12) is both faster and more performant than the {\em single} best performing model (100/4 →  150) by 40 ms. 
}
\label{tab:av2-novel-landscape}
\adjustbox{width=0.85\linewidth}{
\begin{tabular}{@{}cclcccccccc@{}}
\toprule
ID & \quad & \multicolumn{1}{c}{Method}    & 0-50m         & 50-100m              & 100-150m             & 0-150m                       & Runtime (ms)   \\ \midrule% & w/ Post Proc. \\ \midrule
%1 & & 100/4 → 100 (reported by \cite{wilson2021argoverse})  &    24.1          &                      &                      &                          &  \\ \midrule

1 & & 50/8 → 50                            &       31.2          &                      &                 &         17.7                     &    106.9 $\pm$ 0.9      \\ % & 513.3 $\pm$ 49.3\\  
2 & & 50/8 → 100                           &       30.2          &        7.8              &                 &           17.9                   &     399.5 $\pm$  3.2    \\ % & 793.3 $\pm$ 50.3\\
3 & & 50/8 → 150                           &    29.0             &       7.4               &      0.7           &         16.3                     &     900.1  $\pm$ 7.1  \\ \midrule%    & 1290.4 $\pm$ 49.1\\   \midrule

4 & & 100/4 → 50                           &       30.3          &                      &                 &         17.0                     &   37.9 $\pm$ 4.7       \\ %  & 514.9 $\pm$ 53.4\\
5 & & 100/4 → 100                          &     30.1            &     13.2                 &                 &       20.3                       &     104.5 $\pm$ 1.5   \\ %    & 556.2 $\pm$ 51.3\\ 
6 & & 100/4 → 150                          &       30.1          &         13.1             &     5.3            &        20.6                      &     228.0 $\pm$ 1.5  \\ \midrule%    & 665.7 $\pm$ 55.6\\   \midrule

7 & & 150/2 → 50                          &      22.3           &                      &                 &        12.1                      &     16.2 $\pm$ 0.7    \\ % & 132.2 $\pm$ 17.9 \\ 
8 & & 150/2 → 100                         &     22.3            &       11.9               &                 &            15.5                  &     35.9 $\pm$ 0.9   \\ %    & 537.6 $\pm$ 57.8 \\
9 & & 150/2 → 150                         &      22.3           &        11.9              &       5.9          &       15.9                       &      62.0 $\pm$ 0.9  \\ \midrule%    & 540.8 $\pm$ 56.0\\   \midrule

10 & & Range Ensemble  (1,5,9)                &      31.2           &          13.2            &          5.9       &         21.5                     &     273.4 $\pm$ 3.3 \\ %& 1610.3 $\pm$  156.6   \\ 
11 & & + Range Crop                           &      31.2           &          13.2            &          5.9       &         21.5                     &   263.7 $\pm$ 1.9  \\ % &  1392.6 $\pm$ 159.0\\ 
%12 & & + Shared Encoder                           &       \textbf{35.3}            &      \textbf{15.2}                     &         \textbf{6.5}                   &        \textbf{24.4}                         &  \\
%12 & & + Shared Post-Proc.                             &       \textbf{35.3}            &      \textbf{15.2}       %              &         \textbf{6.5}                   &        \textbf{24.4}                         &   \\
12 & & + Near-Far                            &   31.2              &       11.0               &   4.6              &      20.8                        &     185.3 $\pm$ 1.9 \\ \bottomrule%  & 953.0 $\pm$ 159.0\\  \bottomrule

\end{tabular}
} % adjustbox
\end{table*}

\begin{table*}[t]
\small
\centering
\caption{{\bf PointPillars.}  We find the {\em single} best model evaluated over the full range 0-150m is a model trained on the limited range of 50m, but run fully-convolutionally at test time on ranges up to 100m. However, this model essentially gives up on far-field detection (from 100m-150m) and is quite slow. To address both limitations, we build range experts for near, mid, and far field detection. The best performing near-field accuracy arises from a near-range model with high resolution voxels ($50/8 \rightarrow 50$), while the best performing mid-range model makes use of mid-size voxels ($100/4 \rightarrow 100$), and the best far-field detector makes use of low-resolution voxels ($150/4 \rightarrow 150$). The final range ensemble combining all models performs the best. Interestingly, a simple near-far network (that runs far-field detectors at a 3x lower frame rate, using a constant velocity forecaster to estimate object locations for frames without far-field processing) has the second best accuracy overall and outperforms our single best model while running 50ms faster.}
\label{tab:av2-pointpillars-landscape}
\adjustbox{width=0.85\linewidth}{
\begin{tabular}{@{}cclcccccccc@{}}
\toprule
ID & \quad & \multicolumn{1}{c}{Method}    & 0-50m         & 50-100m              & 100-150m             & 0-150m                       & Runtime (ms)  \\ \midrule%& w/ Post Proc. \\ \midrule

%1 & & 50/2 → 50                            &  16.5         &                      &                      &   9.1                        &  75.2 $\pm$ 3.6 \\ 
%2 & & 50/4 → 50                            &  26.8         &                      &                      &   14.9                       &  95.3 $\pm$ 7.4 \\
1 & & 50/8 → 50                            &  \textbf{31.5}&                      &                      &   17.8                      &  61.2 $\pm$ 3.3 \\ %& 121.7 $\pm$ 7.0\\ 
2 & & 50/8 → 100                           &  30.8         &  8.0                 &                      &   19.0                     &   141.6 $\pm$ 2.5\\  %& 226.9 $\pm$ 9.6\\ 
3 & & 50/8 → 150                           &  30.9         &  8.0                 &   0.1                &   18.6                       & 275.8 $\pm$ 2.4\\ \midrule%& 401.0 $\pm$ 4.0\\ \midrule

%6 & & 100/2 → 100                          &  16.9         &  9.3                 &                      &   11.6                       &  84.9 $\pm$ 4.9  \\
4 & & 100/4 → 50                           &  26.7         &                      &                      &   14.9                       &  37.1 $\pm$ 6.0\\ %& 95.3 $\pm$ 7.6\\
5 & & 100/4 → 100                          &  26.9         &  \textbf{13.1}       &                      &   18.2                       &  53.8 $\pm$ 6.2\\ %& 115.8 $\pm$ 7.4\\
6 & & 100/4 → 150                          &  26.9         &  13.1                &   5.2                &   18.2                       &   88.6 $\pm$ 6.5\\ \midrule% & 159.1 $\pm$ 7.6\\ \midrule

7 & & 150/2 → 50                          &   16.7         &                      &                      &   9.2                        &  17.3 $\pm$ 1.2 \\%& 76.1 $\pm$ 3.2\\
8 & & 150/2 → 100                         &   16.7         &  9.3                 &                      &   11.5                       &  22.1 $\pm$ 2.7 \\%& 82.8 $\pm$ 4.6\\
9 & & 150/2 → 150                         &   16.7         &  9.4                 &   \textbf{5.3}       &   12.0                       &  31.6 $\pm$ 3.0 \\ \midrule%& 82.6 $\pm$ 10.1\\ \midrule

10 & & Range Ensemble  (1, 5, 9)         &  \textbf{31.5}         &  \textbf{13.1}                &   \textbf{5.3}                &   \textbf{21.8} &   137.1 $\pm$ 12.0 \\%& 395.9 $\pm$ 24.5\\  
11 & & + Range Crop                             &  \textbf{31.5}         &  \textbf{13.1}                &   \textbf{5.3}                &   \textbf{21.8} &   127.0 $\pm$ 10.0 \\%& 385.8 $\pm$ 24.4\\
%12 & & + Shared Encoder                             &  \textbf{31.5}         &  \textbf{13.1}                &   \textbf{5.3}                &   \textbf{21.8} &   \\
%12 & & + Shared Post Proc.                             &  \textbf{31.5}         &  \textbf{13.1}                &   \textbf{5.3}                &   \textbf{21.8} &  187.3 $\pm$ 14.3\\
13 & & + Near-Far                         &  \textbf{31.5}         &   11.2                        &   4.4         &         21.3         &    94.1 $\pm$ 10.0\\ \bottomrule %& 253.8 $\pm$ 24.4\\ \bottomrule

\end{tabular}
} % adjustbox
\end{table*}

\begin{table*}[t]
\small
\centering
\caption{{\bf CBGS}. The {\em single} best CBGS model is 50/12.5 → 50. As shown with other architectures, this suggests that it is better to ``give up'' on long-range detection. Based on prior analysis in Tab. \ref{tab:av2-novel-landscape}, we posit that the 50m range expert does not generalize across-range well because it only trains on dense regions of the point cloud. Furthermore, we note that CBGS range experts perform best at the range which they are trained. For example, when evaluated between 0-50m, the 100m range expert achieves the highest performance when run at 100m (row 5). Similarly, when evaluated between 0-50m, the 150m range expert achieves the highest performance when run at 150m (row 9). Lastly, the near-far ensemble nearly matches the performance of the range ensemble, but is 33\% faster. 
}
\label{tab:av2-cbgs-landscape}
\adjustbox{width=0.85\linewidth}{
\begin{tabular}{@{}cclcccccccc@{}}
\toprule
ID & \quad & \multicolumn{1}{c}{Method}    & 0-50m         & 50-100m              & 100-150m             & 0-150m                       & Runtime (ms) \\ \midrule%    & w/ Post Proc. \\ \midrule
%1 & & 100/4 → 100 (reported by \cite{wilson2021argoverse})  &    24.1          &                      &                      &                          &  \\ \midrule

1 & & 50/12.5 → 50                            &    \textbf{23.3}           &               &                      &      \textbf{13.4}   &  52.5 $\pm$ 3.4 \\ %& 118.5 $\pm$ 10.4\\ 
2 & & 50/12.5 → 100                           &    21.7           &   6.6         &                      &     13.3                      &  76.3 $\pm$ 2.5 \\ %& 135.3 $\pm$ 3.6\\ 
3 & & 50/12.5 → 150                           &    21.0           &   5.9         &   1.2                &      12.1                     &  113.7 $\pm$ 2.5 \\ \midrule%& 178.0 $\pm$ 3.9\\  \midrule

4 & & 100/6.25 → 50                           &     13.1          &               &                      &    7.6                        &  44.1 $\pm$ 1.1  \\ %& 102.6 $\pm$ 2.8\\
5 & & 100/6.25 → 100                          &   15.4            &     \textbf{7.1}       &                      &    10.3                       &  48.7 $\pm$ 2.0 \\ %& 85.1 $\pm$ 9.1\\
6 & & 100/6.25 → 150                          &    13.3           &    6.2        &   \textbf{2.8}                &    9.0                        &  57.4 $\pm$ 1.8 \\ \midrule%& 88.4 $\pm$ 5.6\\  \midrule

7 & & 150/3.125 → 50                           &    4.5              &                      &                      &  2.7                      &  40.5 $\pm$ 0.6  \\ %& 97.3 $\pm$ 1.7\\ 
8 & & 150/3.125 → 100                          &    2.7              &      1.4                &                      &    1.9                    & 40.9 $\pm$ 1.0  \\ %& 99.7 $\pm$ 2.8\\ 
9 & & 150/3.125 → 150                          &   5.5            &     2.8              &     1.7              &     3.8                &  41.7 $\pm$ 1.1 \\ \midrule%& 100.5 $\pm$ 2.7\\  \midrule

10 & & Range Ensemble (1, 5, 6)                      &    \textbf{23.3}              &      \textbf{7.1}                      &     \textbf{2.8}                 &   \textbf{15.2}                           &  154.0 $\pm$ 7.2 \\ %& 292.0 $\pm$ 25.1\\ 
11 & & + Range Crop                             &    \textbf{23.3}              &     \textbf{7.1}                      &     \textbf{2.8}                 &   \textbf{15.2}                           &  148.0 $\pm$ 10.3\\ 
%12 & & + Shared Post-Proc.                             &    \textbf{23.3}              &     \textbf{7.1}          %            &     \textbf{2.8}                 &   \textbf{15.2}                           &  \\ 
%13 & & + Shared Post-Proc.                             &    \textbf{23.3}              &     \textbf{7.1}                      &     \textbf{2.8}                 &   \textbf{15.2}                           &  \\ 
13 & & + Near-Far                         &     \textbf{23.3}                   &     5.8                          &    2.3                           &     15.0           &   100.3 $\pm$  10.3 \\\bottomrule

\end{tabular}
} % adjustbox
\end{table*}

\begin{table*}[t]
\small
\centering
\caption{{\bf CenterPoint}. Evaluating both the 100m  and 150m range experts, we find that both models generalize across-range.  In contrast, we find that the  50m range expert does not generalize well, suggesting that across-range generalization is both a property of training range and voxel size. Concretely, training only with dense near-field LiDAR points or fine-grained voxels won't generalize well at long-range with sparse LiDAR-points. Surprisingly, the CenterPoint range ensemble does not make use of the 50m range expert. This suggests that smaller voxels does not guarantee better performance. Particularly, the best 100m range expert (100/6.25 →  150) achieves nearly 5 \% CDS greater than the best 50m range expert (50/12.5 →  100). Finally, we note that the near-far ensemble (row 12) is both faster and more performant than the {\em single} best performing model (100/6.25 →  150) by 20 ms. 
}
\label{tab:av2-centerpoint-landscape}
\adjustbox{width=0.85\linewidth}{
\begin{tabular}{@{}cclcccccccc@{}}
\toprule
ID & \quad & \multicolumn{1}{c}{Method}    & 0-50m         & 50-100m              & 100-150m             & 0-150m                       & Runtime (ms)   \\ \midrule% & w/ Post Proc. \\ \midrule
%1 & & 100/4 → 100 (reported by \cite{wilson2021argoverse})  &    24.1          &                      &                      &                          &  \\ \midrule

1 & & 50/12.5 → 50                            &   32.7          &                      &                 &    19.0                         &  92.4 $\pm$ 5.1 \\ %& 493.6 $\pm$ 48.2\\  
2 & & 50/12.5 → 100                           &   31.9          &    7.8               &                 &        19.8                     &  239.7 $\pm$ 5.1 \\ %& 659.2 $\pm$ 47.5\\ 
3 & & 50/12.5 → 150                           &   31.6          &    7.6               &     1.0         &      19.1                       &  492.2 $\pm$ 6.1 \\ \midrule%& 908.6 $\pm$ 47.9\\   \midrule

4 & & 100/6.25 → 50                           &     \textbf{35.3}        &                      &                 &            19.9                 &  56.3 $\pm$ 3.8 \\ %& 533.0 $\pm$ 50.8\\ 
5 & & 100/6.25 → 100                          &  35.2           &   \textbf{15.2}               &                 &        24.0                     &  91.0 $\pm$ 5.8 \\ %& 245.8 $\pm$ 33.0\\ 
6 & & 100/6.25 → 150                          &     35.2        &       \textbf{15.2}           &    6.1          &         24.3                    &  152.2 $\pm$ 4.8\\ \midrule%& 592.5 $\pm$ 56.9\\   \midrule

7 & & 150/3.125 → 50                           &    25.9           &                      &                  &       14.2                          & 48.6 $\pm$ 5.5  \\ %& 163.1 $\pm$ 22.7\\ 
8 & & 150/3.125 → 100                          &    26.0           &    12.3                  &                  &   17.7                              &  52.7 $\pm$ 3.7 \\ %& 522.7 $\pm$ 57.4\\ 
9 & & 150/3.125 → 150                          &    26.0       &     12.3             &   \textbf{6.5}           &       18.3                      &  68.6 $\pm$ 3.2 \\ \midrule% & 355.0 $\pm$ 68.1\\   \midrule

10 & & Range Ensemble  (4,5,9)                     &       \textbf{35.3}            &      \textbf{15.2}                     &         \textbf{6.5}                   &        \textbf{24.4}                         & 215.9 $\pm$ 13.3 \\ 
11 & & + Range Crop                             &       \textbf{35.3}            &      \textbf{15.2}                     &         \textbf{6.5}                   &        \textbf{24.4}                         &  208.2 $\pm$ 13.9\\
%12 & & + Shared Encoder                           &       \textbf{35.3}            &      \textbf{15.2}                     &         \textbf{6.5}                   &        \textbf{24.4}                         &  \\
%12 & & + Shared Post-Proc.                             &       \textbf{35.3}            &      \textbf{15.2}       %              &         \textbf{6.5}                   &        \textbf{24.4}                         &   \\
12 & & + Near-Far                         &        35.3              &    12.8                     &      4.6                         &     23.6           &  132.3 $\pm$ 13.9  \\  \bottomrule

\end{tabular}
} % adjustbox
\end{table*}

\begin{table*}[t]
\small
\centering
\caption{{\bf TransFusion-L}. We evaluate TransFusion-L across ranges using fully convolutional processing but find that the model does not generalize across-ranges. For example, the 50m expert achieves 23.4 CDS when run at 50m (row 1), but loses 15\% CDS when run at 100m and achieves 0\% DS when run at 150m. Similarly, the 100m range expert attains 21.1 CDS when run at 100m (row 5), but achieves nearly 0\% CDS when run at either 50m or 150m. We posit that using metric positions for positional encoding rather than relative positions may yield better across-range generalisation. We find that the TransFusion range ensemble (row 10) has the highest performance of all architectures. Next, we find that the ``donut-shaped'' range crop significantly improves the efficiency of the range ensemble. Laslty, the near far ensemble achieves nearly the same performance as range ensemble but is 33\% faster.
}
\label{tab:av2-transfusion-landscape}
\adjustbox{width=0.85\linewidth}{
\begin{tabular}{@{}cclcccccccc@{}}
\toprule
ID & \quad & \multicolumn{1}{c}{Method}    & 0-50m         & 50-100m              & 100-150m             & 0-150m                       & Runtime (ms)   \\ \midrule% & w/ Post Proc. \\ \midrule
%1 & & 100/4 → 100 (reported by \cite{wilson2021argoverse})  &    24.1          &                      &                      &                          &  \\ \midrule

1 & & 50/12.5 → 50                            &  \textbf{40.9}               &                      &                 &       23.4                      &  280.9  $\pm$ 22.0 \\ %& 282.4 $\pm$ 22.5 \\  
2 & & 50/12.5 → 100                           &  13.7               &    1.1                  &                 &           
   7.8               & 332.7 $\pm$  21.7 \\ %&  334.1 $\pm$ 21.9\\  
3 & & 50/12.5 → 150                           &   0.0              &     0.0                 &     0.0            &            0.0                 &  410.7 $\pm$  19.7  \\ \midrule%& 412.2 $\pm$ 19.8 \\  \midrule

4 & & 100/6.25 → 50                           &   1.6              &                      &                 &         1.0                    & 256.5 $\pm$ 20.5 \\ %& 258.1 $\pm$ 21.1 \\  
5 & & 100/6.25 → 100                          &   34.5              &     \textbf{8.2}                 &                 &     21.1                        & 273.1 $\pm$  17.2 \\ %& 274.5 $\pm$ 19.7 \\  
6 & & 100/6.25 → 150                          &   1.0              &     0.2                 &      0.0           &       0.6                      & 288.5 $\pm$  19.9 \\ \midrule%& 291.0 $\pm$ 20.3 \\  \midrule

7 & & 150/3.125 → 50                           &    2.2           &                      &                  &                1.2                 & 239.8 $\pm$  21.0 \\ %& 241.5 $\pm$ 21.7 \\ 
8 & & 150/3.125 → 100                          &    0.9           &      0.3                &                  &        0.6                         & 254.3 $\pm$  18.0 \\ %& 255.9 $\pm$ 18.5 \\ 
9 & & 150/3.125 → 150                          &    19.8             &   4.5                   &      0.0           &    11.7                         &  253.5 $\pm$ 16.3\\ \midrule% & 256.0 $\pm$  16.9 \\  \midrule

10 & & Range Ensemble  (1, 5)                         &      40.9           &    8.2                  &      0.0           &           \textbf{25.1}                  &  556.9 $\pm$ 42.2 \\ %& 558.3 $\pm$ 44.1\\  
11 & & + Range Crop                             &      40.9           &    7.4                  &      0.0           &           24.8                  &   436.6 $\pm$ 66.6 \\ %& 438.2 $\pm$ 63.1 \\ %
%12 & & + Shared Encoder                         &      40.9           &    7.4                  &      0.0           &           24.8                  &   \\ 
%12 & & + Shared Post Proc.                      &      40.9           &    7.4                  &      0.0         %  &           24.8                  &   \\ 
12 & & + Near-Far                         &     40.9                   &       6.8                        &    0.0                           &    24.7            &   361.2 $\pm$ 66.6 \\ \bottomrule%& 363.5 $\pm$ 63.1 \\  \bottomrule

\end{tabular}
} % adjustbox
\end{table*}
